# Supplementary material for: Single neutral pion production by charged-current $\bar{\nu}_\mu$ interactions on hydrocarbon at $\langle E_\nu \rangle = $ 3.6 GeV
Source: arXiv:1503.02107 source file (2015-08-25)
Supplement: Supplementary file 1 [file supplement.tex]

%% TO CHECK LENGTH... go to ``review and submission option'' and set
%%``sizecheck'' to ``1'' below.  Remember to unset when done!

%% for review and submission
\documentclass[aps,prl,twocolumn,showpacs,superscriptaddress,nofootinbib]{revtex4}

%% for double-spaced preprint

%\documentclass[aps,prl,preprint,showpacs,superscriptaddress,linenumbers]{revtex4} 

\usepackage{amsmath}   % need for subequations
\usepackage{graphicx}  % for figures
\usepackage{xspace}
\usepackage{units}

\usepackage{hyperref}

 % 0 to do nothing; 1 to check size

%ability to convert eps to pdf at compile time
\newif\ifpdf
\ifx\pdfoutput\undefined
   \pdffalse
\else
   \pdfoutput=1
   \pdftrue
\fi
\ifpdf
   \usepackage{graphicx}
   \usepackage{epstopdf}
   \DeclareGraphicsRule{.eps}{pdf}{.pdf}{`epstopdf #1}
   \pdfcompresslevel=9
\else
   \usepackage{graphicx}
\fi

\begin{document}

\thispagestyle{empty}

\input{appendix.tex}

\end{document}
